# Supplementary material for: Learning functional programs with function invention and reuse
Source: arXiv:2011.08881 source file (2020-11-17)
Supplement: Supplementary file 1 [file appendixa.tex]

\chapter{Implementation details}

We briefly give some implementation details for the system.  The full code can be found at the address: https://github.com/AndreiDiaconu1/inductive-haskell. We have two implementations, one for each of the presented algorithms. They both share the language and type system, the main difference being the file \textit{Search.hs}, which contains the implementations of the search algorithm.

\section{Language implementation}
The language that we have presented in chapter 4 is very similar to the language Fun, presented in the POPL course \cite{popl}. Hence, we have used the parser and lexer, together with parts of the evaluator for our implementation, but we have extended them with new constructs. We have added types to the language and added a type inference system (which can be found in the file \textit{Infer.hs}). The inference algorithm follows classical implementations, being very similar to $Algorithm \mathcal{W}$ and a similar explained implementation can be found at . To support the synthesis process inside the language, we have added three constructs to the language presented in chapter 4: 
\begin{itemize}
\item \textit{PEx} \textbf{ins} => \textbf{out}:  
\item \textit{PEx} \textbf{ins} => \textbf{out}: 
\item \textit{Synthesize} \textbf{type}: this is used to start the synthesis process, specifying that the expected type is \textbf{type}
\end{itemize}
Listing A.1 shows the test file used for \textit{maze}, which highlights all the features of the language.
\begin{lstlisting}[frame=single, caption=maze.test]
val comp(f, g) = lambda (x) f(g(x)) ;;

rec map(f) = lambda (xs)
    (if xs = nil
    then nil
    else f(head(xs)):map(f)(tail(xs))) ;;

rec filter(p) = lambda (xs)
    (if xs = nil
    then nil
    else 
        if (p(head(xs)))
        then head(xs):filter(p)(tail(xs))
        else filter(p)(tail(xs))) ;;

val BK_addOne(x) = x + 1 ;;

NEx (1) => 2 ;;
NEx (3) => 5 ;;
PEx (1) => 9 ;;
PEx (7) => 15 ;;
Synthesize (Int) => Int;;
\end{lstlisting}

\section{Algorithms implementation}
We have written two distinct implementation for the algorithms. Generally, the two algorithms are direct implementations of the algorithm. They can be found in the file \textit{Search.hs}.

\iffalse
\begin{lstlisting}[frame=single, caption=progSearch]
progSearch :: (ProgState -> Bool) -> 
              (ProgState -> [ProgState]) -> 
              ProgState -> Maybe IProgram
progSearch check expand init = 
    selectFirstResult (\d ->  dbSearch d check expand init) [1 .. ]
    -- stopFound makes sure we stop
    -- when the first valid node has been
    -- checked and produced a valid
    -- result
    where dbSearch d check next crtState
            | d == 0 = Nothing
            | check crtState == True  = Just (getIProgram crtState)
            | check crtState == False = 
                 stopFound (dbSearch (d - 1) check next) (next crtState)
\end{lstlisting}

\begin{lstlisting}[frame=single, caption=expand]
expand :: ProgState -> [ProgState]
expand (ip, pinf)  
    -- onlyValid retrieves the legal filled 
    -- definitions
    | not (isCompleteIP ip) = onlyValid filledDefns
    -- if the program is complete, 
    -- nothing to expand
    | otherwise = []
    where
        -- defn should have an Empty body that
        -- awaits a a metarule application
        (defn, newIProg) = getAnIncomplete ip
        withMetarules = applyMetarules defn (pinf.metarules)
        -- onlyNames will contain a list of the names 
        -- that we have been user provided or 
        -- previously synthesized
        onlyNames = getBackgroundInfoNames pinf 
        -- the getCartesianProduct function gets
        -- all possible combinations of the available
        -- functions and the newly invented functions
        -- (i.e. we create fresh names);
        -- those new functions are added to the
        -- typing environment by updatePinf
        -- using fresh type variables;
        filledDefns = 
         [ fill (updatePInf pinf toFillWith) def toFillWith  | 
           afterMrApply <- withMetarules, 
           toFillWith <- getCartesianProduct onlyNames]
\end{lstlisting}
\fi
